# Supplementary material for: Quantifying Energetic and Entropic Pathways in Molecular Systems
Source: arXiv:2203.07560 ancillary file (2022-03-14)
Supplement: Supplementary file 1 [file supplement.pdf]

# Supplementary Material for "Quantifying Energetic and Entropic pathways in Molecular Systems"

E. R. Beyerle
*Institute for Physical Science and Technology, University of Maryland, College Park, Maryland 20740, USA*

Shams Mehdi
*Biophysics Program and Institute for Physical Science and Technology,*
*University of Maryland, College Park 20742, USA*

Pratyush Tiwary*
*Department of Chemistry and Biochemistry and Institute for Physical Science and Technology,*
*University of Maryland, College Park 20742, USA*
(Dated: March 14, 2022)

* ptiwary@umd.edu

## I. SIMULATION DETAILS FOR BA-DMPC SYSTEM

CHARMM-GUI [1] was used to generate the force field parameterization for the lipid groups while the benzoic acid molecule was parameterized using CGenFF [2]. Each side of the DMPC bilayer is composed of 40 lipids, and the entire BA-DMPC system is solvated with 71,102 TIP3P water molecules. A snapshot of the final, solvated system is shown in Figure S1(a) where the benzoic acid is inside the bilayer. Figure S1(b) shows an ensemble of snapshots of benzoic acid from the simulation, showing that, when the benzoic acid molecule is sufficiently close to the underside of either side of the bilayer, it preferentially orients the -COOH group toward the DMPC headgroups on that side of the membrane, in agreement with the free-energy surface for this system shown in Figure 6 of the main text.

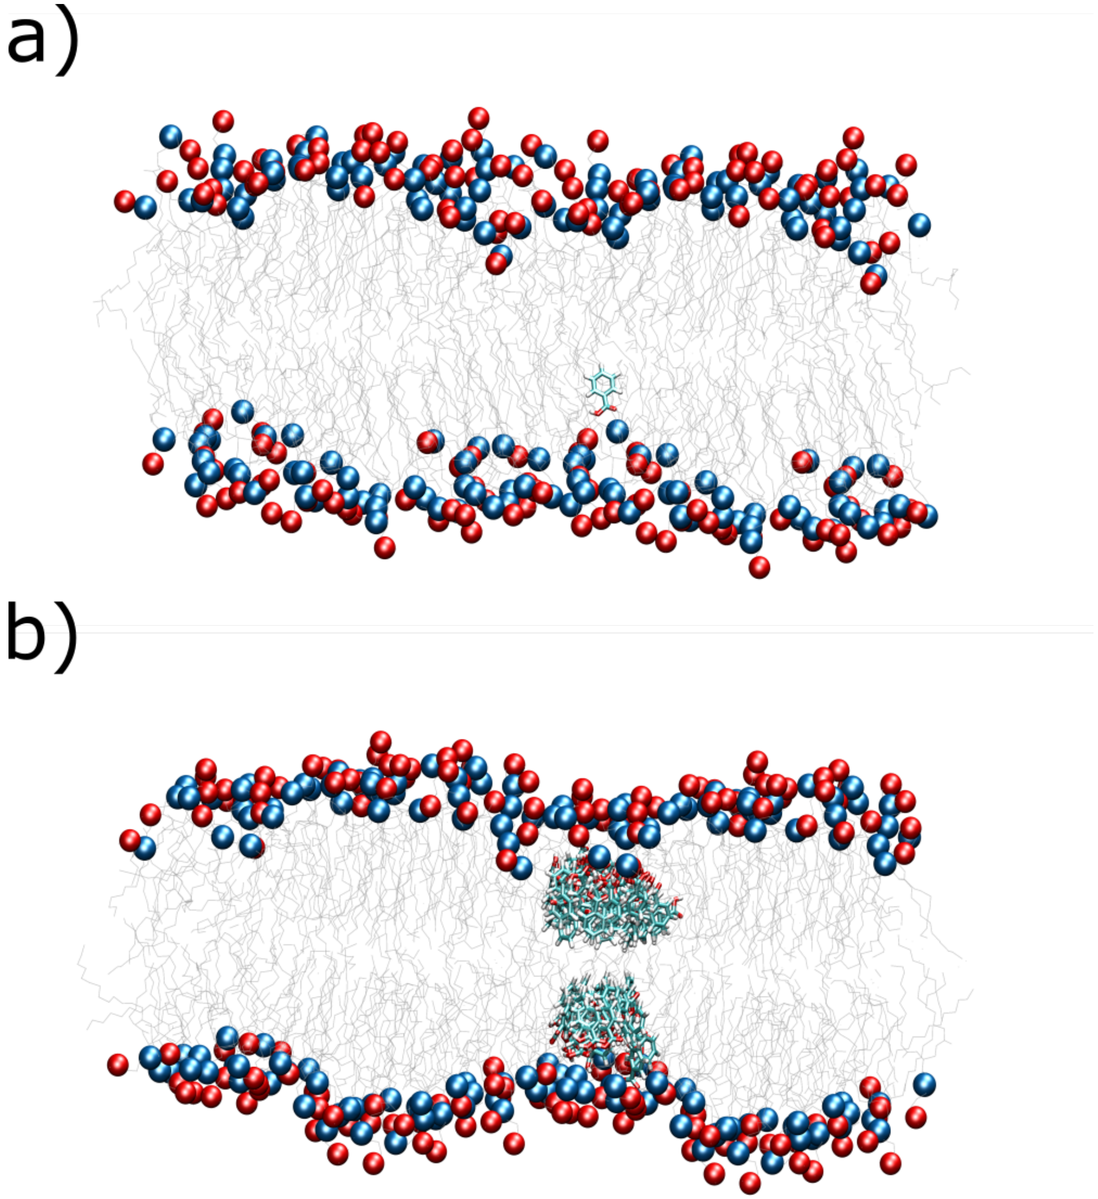


FIG. S1. Panel a: Snapshot of benzoic acid (licorice representation) inside the DMPC bilayer. The hydrophobic tails of DMPC are represented as grey sticks while the nitrogen and phosphorous atoms in the headgroups are represented as red and blue spheres, respectively. Panel b: An ensemble of snapshots from the BA-DMPC simulation for a biased trajectory equaling 500 ns in duration showing the preferential orientation of the -COOH group of benzoic acid when proximate to the underside of each DMPC leaflet.

The simulation is performed in the NPT ensemble with the temperature set to 298.15 K using the Nosé-Hoover

thermostat[3] and the pressure set to 1 bar using the Parrinello-Rahman barostat[4]. The position of each atom in the system were saved to file every 0.2 ps. As described in the main text, two initial simulations of 25 ns each, where the benzoic acid was placed on opposite sides of the bilayer in either simulation, were run to find an initial one-dimensional SPIB reaction coordinate, and the combined trajectories from these simulations were then used to run a 500 ns simulation biased along this SPIB coordinate. The same thermodynamic conditions were used in both the unbiased and biased simulation runs, and the biasing was performed using well-tempered metadynamics [5] as implemented in PLUMED version 2.6.2 [6]. Because the BA-DMPC simulation analyzed comes from a biased trajectory, when calculating thermodynamic quantities and constructing free-energy surfaces for this system, all trajectory points are re-weighted using the time-dependent metadynamics bias, as described in detail in, e.g., [7, 8]. All simulations were performed using GROMACS 2020.2[9] patched with PLUMED 2.6.2[6]. Other details of the MD simulation for this system and the detailed definitions of the 21 order parameters input to the SPIB analysis can be found in ref. [10].

## II. SPIB ANALYSIS DETAILS

Table S1 details the SPIB parameters used for the entropic double well, temperature switch, and BA-DMPC systems analyzed in the main text.

TABLE S1. SPIB analysis details for the entropic double well (EDW), temperature-switch (TS) potentials, and benzoic acid permeation through the DMPC bilyer (BA-DMPC)

| Parameter | EDW | TS | BA-DMPC |
|---|---|---|---|
| s[a] | 1500 | 5 | 200[a] |
| $\beta$ | 0.025 | 0.01 | 0.2 |
| learning rate[b] | 0.001 | 0.001 | 0.005 |
| # neurons[c] | 16 | 64 | 64 |
| K | 10 | 10 | 7 |

[a]Units of $\Delta t$ for TS and EDW; units of ps for BA-DMPC.
[b]TS and BA-DMPC also used a learning rate decay of 0.9 and 0.98, respectively.
[c]Same number of neurons in the encoder and decoder layers.

## III. TICA RESULTS FOR THE TEMPERATURE SWITCH POTENTIAL

To compare to a ‘control’ analysis, TICA was performed on the temperature switch trajectory using a lagtime of $\tau = 10\Delta t$. The projection of the two TICs onto the temperature switch free-energy surface is shown in Figure S2(a),(b) and the one-dimensional free-energy profile projected along each TIC is given in Figure S2(c),(d). In this instance, the TICA trivially returns the x- and y-coordinates as the two slow coordinates, in that order. The first TIC describes transitions in the x-direction across the primarily entropic bottleneck, while the second TIC describes transitions along the y-direction across the primarily energetic barrier. For the barrier in the x-direction, the magnitude of the energetic and entropic contributions to the overall free-energy barrier are similar, but the transitions along the y-coordinate, described by the second TICA coordinate, the barrier is dominated by the energetic contribution. For this system, the TICA fails to give any additional insight to the dynamics on the surface, excepting estimates of the kinetics of transitions in the x- and y-directions, which are neither calculated nor reported here.

## IV. TICA RESULTS FOR THE BA-DMPC SYSTEM

For this system as well the SPIB reaction coordinates are compared to the two slowest TICA coordinates. The projection of the two slowest TICs onto the free-energy surface given in Figure 6 of the main text is shown in Figure S3(a),(b) and the decomposition of the free-energy along the two TICs is given in Figure S3(c),(d). The same 21 OPs input to the SPIB analysis were also input to the TICA, and a lagtime of $\tau = 2$ ps was selected for the TICA. Similar to the temperature switch, the first TIC is essentially equivalent to transitions along $d_{1,z}$, and it contains both the entropic barriers at the surface of the membrane and the energetic barrier at the center of the bilayer. The second TIC is fairly nonsensical from a mechanistic perspective, describing transitions in $\theta_z$ at all values of $d_{1,z}$. It is possible that the second TIC is ‘confused’ by the other 19 OPs not represented in the shown two-dimensional free-energy surface, and that, if projected in higher dimensions or if a more judicious two-dimensional surface is selected, then

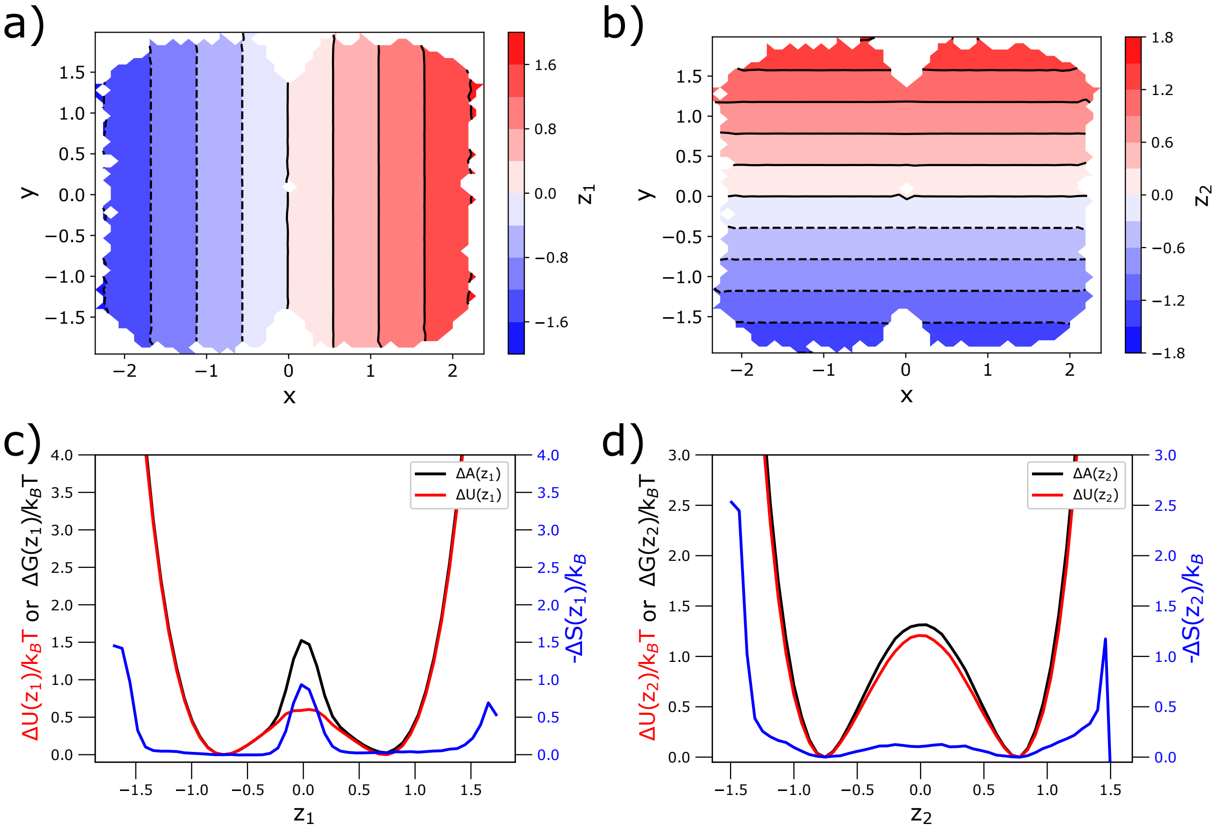


FIG. S2. Panel a: projection of the first TIC, which is essentially equivalent to the y-coordinate, onto the temperature switch free-energy surface. Panel b: projection of the second TIC, which is essentially equivalent to the x-coordinate, onto the temperature switch free-energy surface. Panel c: decomposition of the free-energy profile (black) along the first TIC into its energetic (red) and entropic (blue) components. Based on this decomposition, it is clear the barrier along the first TIC is dominated by the energetic component of the free-energy.. Panel d: decomposition of the free-energy profile (black) along the second TIC into its energetic (red) and entropic (blue) components. Based on this decomposition, the free-energy barrier along the second TIC is roughly equally balanced between the energetic and entropic components.

the second TIC will be more sensible from a physical perspective. However, in either case, TICA is not able to find a set of collective variables that separate the relevant energy and entropy barriers present in the system.


[1] J. Lee, X. Cheng, J. M. Swails, M. S. Yeom, P. K. Eastman, J. A. Lemkul, S. Wei, J. Buckner, J. C. Jeong, Y. Qi, S. Jo, V. S. Pande, D. A. Case, C. L. Brooks, A. D. MacKerell, J. B. Klauda, and W. Im, Journal of Chemical Theory and Computation **12**, 405 (2016).

[2] K. Vanommeslaeghe, E. Hatcher, C. Acharya, S. Kundu, S. Zhong, J. Shim, E. Darian, O. Guvench, P. Lopes, I. Vorobyov, and A. D. Mackerell Jr., Journal of Computational Chemistry **31**, 671 (2010), https://onlinelibrary.wiley.com/doi/pdf/10.1002/jcc.21367.

[3] W. G. Hoover, Phys. Rev. A **31**, 1695 (1985).

[4] M. Parrinello and A. Rahman, Journal of Applied Physics **52**, 7182 (1981).

[5] A. Barducci, G. Bussi, and M. Parrinello, Phys. Rev. Lett. **100**, 020603 (2008).

[6] G. A. Tribello, M. Bonomi, D. Branduardi, C. Camilloni, and G. Bussi, Computer Physics Communications **185**, 604 (2014), arXiv:1310.0980.

[7] G. Bussi, D. Branduardi, *et al.*, Rev. Comput. Chem **28**, 1 (2015).

[8] G. Bussi and G. A. Tribello, in *Biomolecular Simulations* (Springer, 2019) pp. 529–578.

[9] M. J. Abraham, T. Murtola, R. Schulz, S. Páll, J. C. Smith, B. Hess, and E. Lindah, SoftwareX **1-2**, 19 (2015), arXiv:arXiv:1503.05249v1.

[10] S. Mehdi, D. Wang, S. Pant, and P. Tiwary, "Accelerating all-atom simulations and gaining mechanistic understanding of biophysical systems through state predictive information bottleneck," (2021), arXiv:2112.11201 [physics.bio-ph].

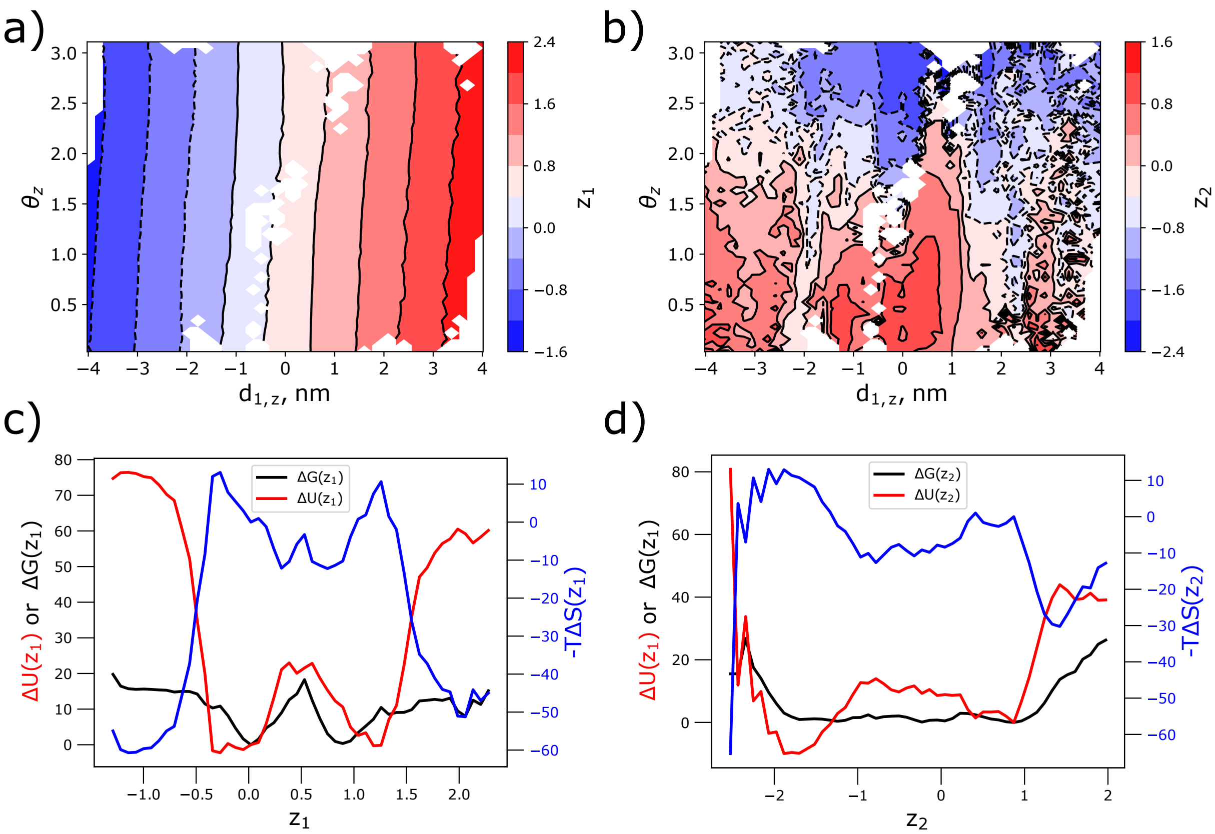


FIG. S3. Panel a: projection of the first TIC, which essentially describes transitions along $d_{1,z}$, onto the two-dimensional BA-DMPC free-energy surface. Panel b: projection of the second TIC onto the two-dimensional BA-DMPC free-energy surface. This coordinate describes transitions from high to low values of $\theta_z$ along the $d_{1,z}$ coordinate. Panel c: projection of the free-energy (black), enthalpy (red), and entropy (blue) along the first TIC. The first TIC captures both the relevant energetic barrier at the center of the bilayer and the entropic barriers on both the exterior sides of the bilayer. Panel d: same as the left panel, except for the second TIC. Units of $\Delta G$, $\Delta U$, and $T\Delta S$ are kJ/mol.
